# Supplementary material for: Parameter-Efficient and Memory-Efficient Tuning for Vision Transformer: A Disentangled Approach
Source: arXiv:2407.06964 source file (2024-07-14)

CLS Token

VQT

SynQT

SVHN  
(Natural)

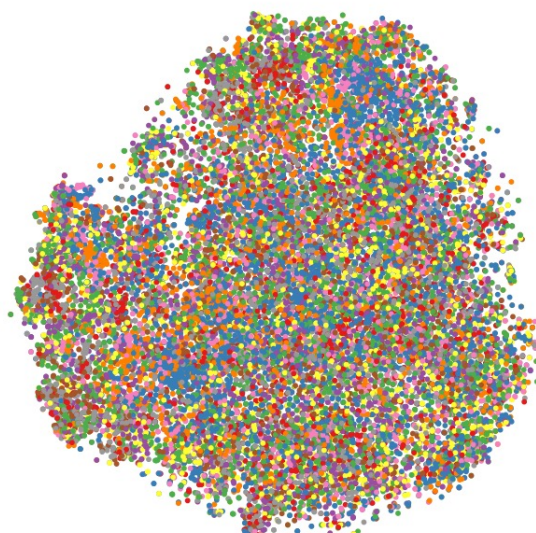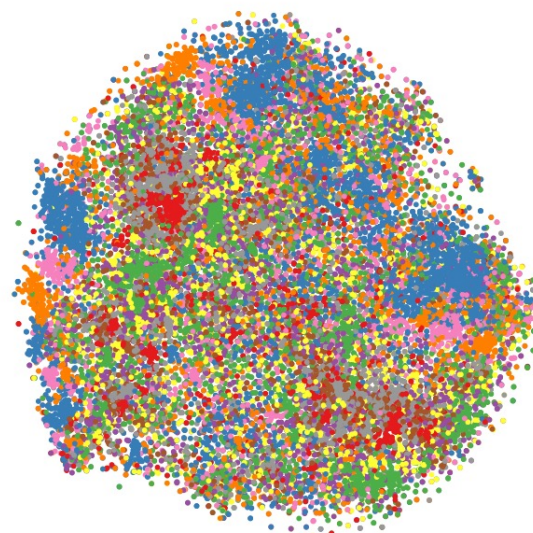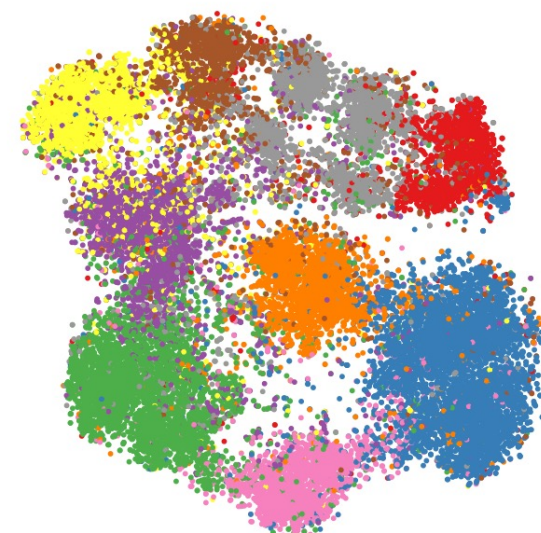

EuroSAT  
(Specialized)

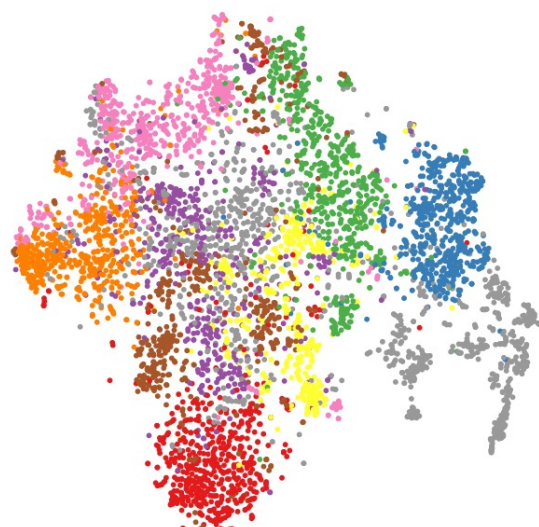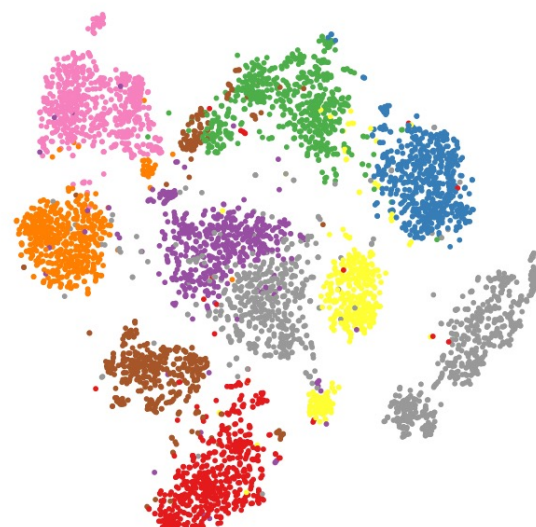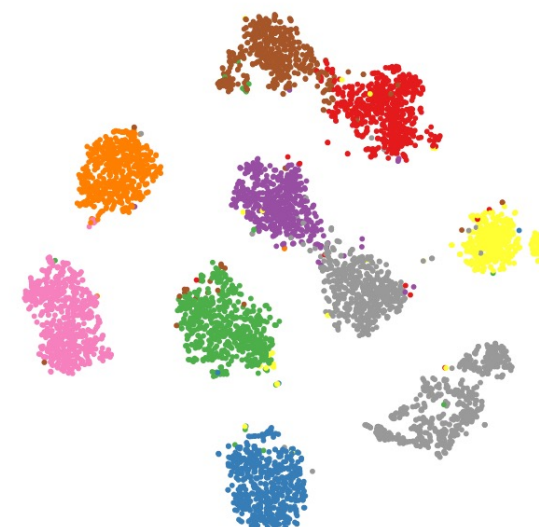

Clevr-Dist  
(Structured)

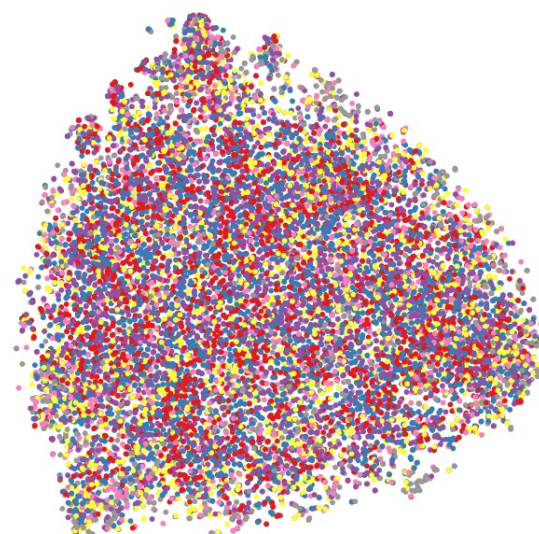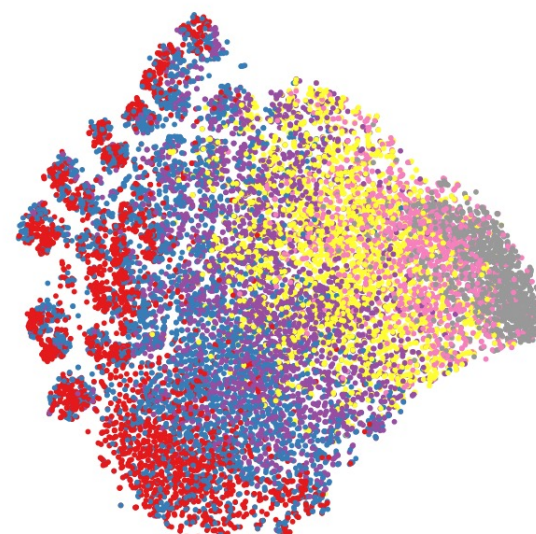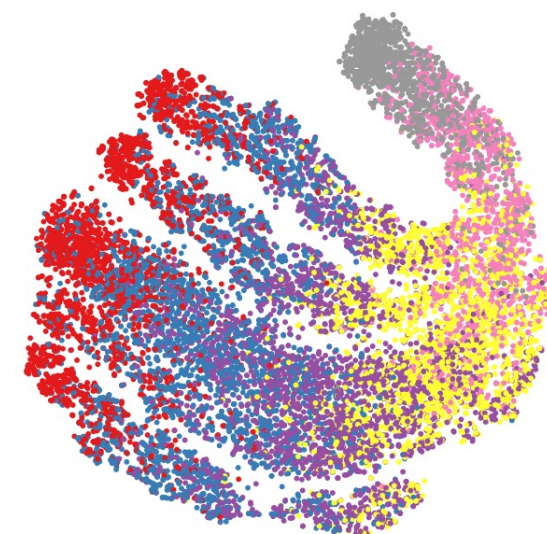



CLS Token

VQT

SynQT

Clevr-Count  
(Structured)

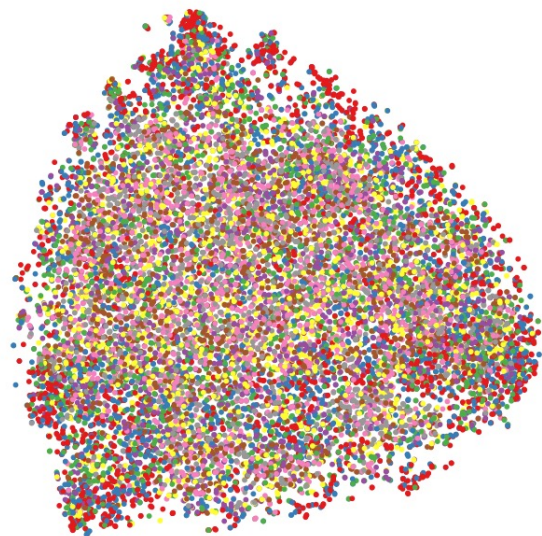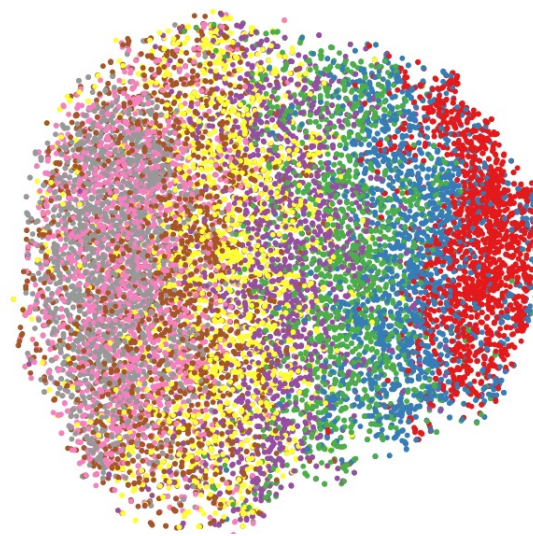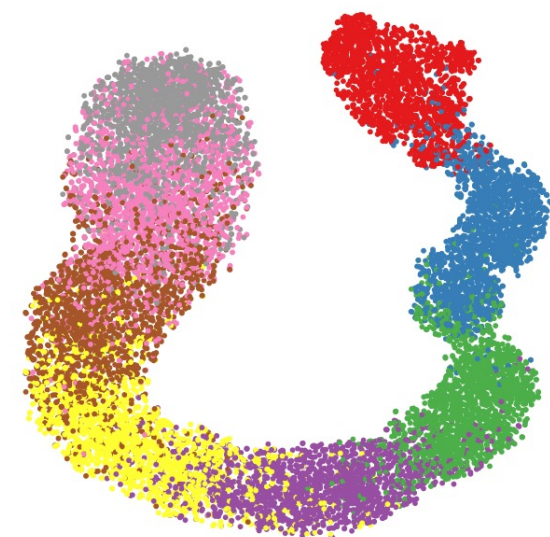

DMLab  
(Structured)

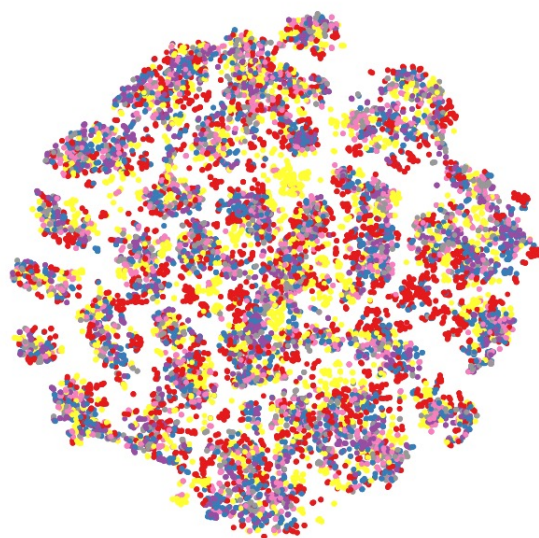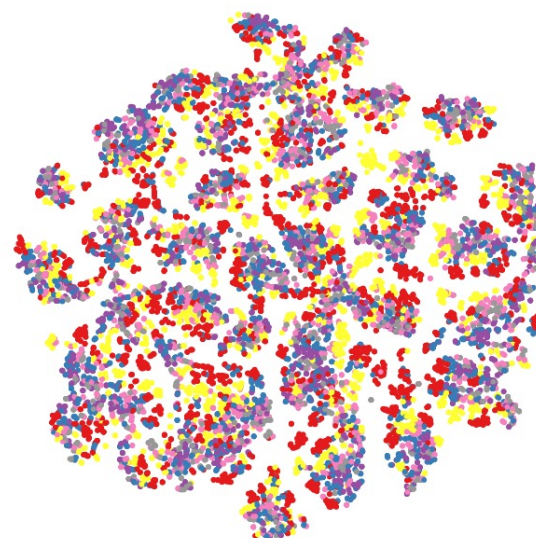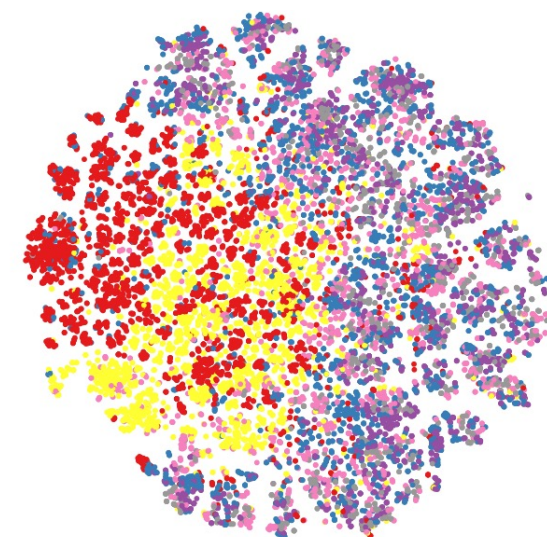

sNORB-Ele  
(Structured)

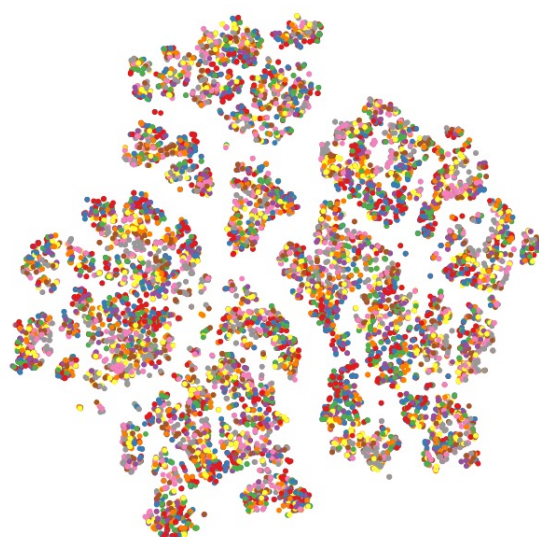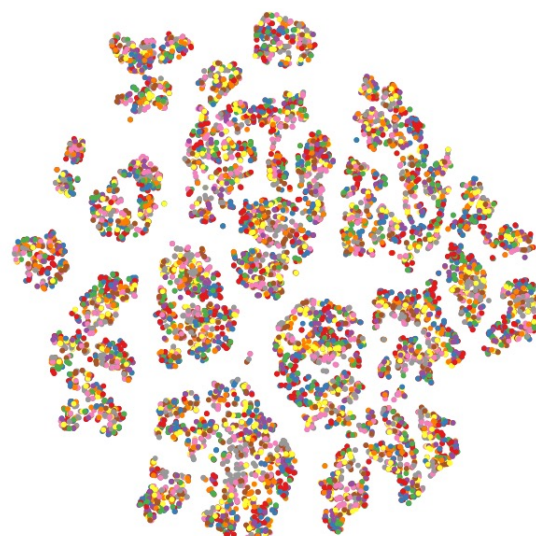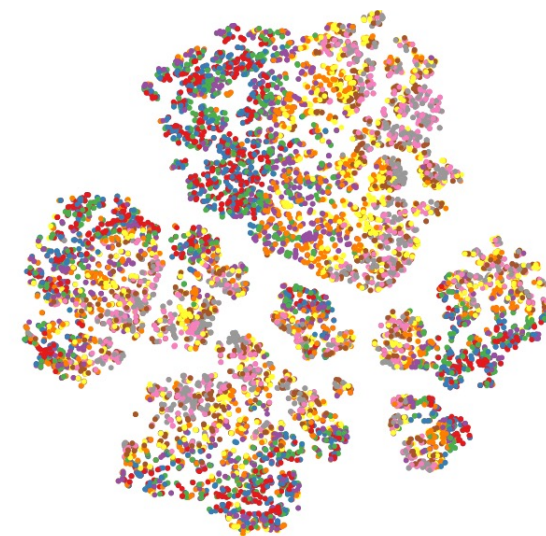

Supplement: Supplementary file 1 [file tsne_appendix.pdf]
