# Supplementary material for: Parameter-Efficient and Memory-Efficient Tuning for Vision Transformer: A Disentangled Approach
Source: arXiv:2407.06964 source file (2024-07-14)
Supplement: Supplementary file 2 [file X_suppl.tex]

\clearpage
\setcounter{page}{1}
\maketitlesupplementary

\section{Analysis on Inference Speed}
The inference speed of the model, influenced by the number of trainable parameters and the architectural design, is important in real-world transfer applications. SynQT, with its lightweight architectures including QSM and KEM, could potentially introduce additional inference costs. Therefore, we evaluate the inference time compared with traditional PETL methods and present the results along with the optimal tokens in Table \ref{tab:time}.

Notably, the inference speed of VPT-Shallow \cite{jia2022visual} is quite slow, as its optimal tokens on CIFAR100 reachs up to 100. In contrast, the inference speeds of BitFit \cite{zaken2021bitfit}, VPT-Deep \cite{jia2022visual}, VQT \cite{tu2023visual}, and SynQT are similar without any significant differences. This suggests that the important factor affecting inference time is the number of prompt tokens rather than the additional lightweight architectures. Given that we use an extremely small number of tokens, with the number range from $\{1,4,16\}$ for the lightweight design of QSM, the overall inference time of SynQT is comparable to VQT and the additional inference cost is affordable.

\input{exp_result/appendix_time.tex}

\section{t-SNE Visualization for More Datasets}
We provide t-SNE \cite{van2008visualizing} visualization for more datasets in Figure \ref{fig:tsne_appendix}. The visualization shows that the features obtained by SynQT is more separable.  
\begin{figure}[htbp]
    \centering
    \includegraphics[width=0.5\textwidth, page=2]{pdf/tsne_appendix.pdf}
    \vspace{-1em}
    \caption{\textbf{t-SNE visualization on more datasets including Clevr-Count, DMLab and sNORB-Ele.}
    % \red{Eurosat to EuroSAT, CLEVR/distance to Clevr-Dist, make all statements consistent!!!!! double-check all statements!!!! suggestion: Cls token to CLS Token; change the sequence of eurosat and svhn; EuroSAT to EuroSAT (Specialized) ... also for svhn and clevr, two lines}
    }
    \vspace{-1.5em}
    \label{fig:tsne_appendix}
\end{figure}

\section{Discussion on Trainable Prameters}
SynQT outperforms previous PETL methods while requiring slightly more trainable parameters. To validate that the superior performance of our method is not due to the additional parameters, we match the numbers of tunable parameters used in VPT-Deep \cite{jia2022visual} and VQT \cite{tu2023visual}, and increase their input tokens to 300.
We term the augmented version of VPT-Deep and VQT as VPT-Deep-Aug and VQT-Aug, respetively.
The comparison between SynQT and these models are provided in Table \ref{tab:parameters}.

As can be seen from the results, increasing the number of tokens does not necessarily yield a significant enhancement in model performance, and may even results in a significant performance drop. The result is consistent with the conclusion in the original paper that the optimal prompt length should not be too large, as the increase in model complexity could cause overfitting due to the limited data on VTAB-1k.

In contrast, SynQT utilizes a maximum of only 16 tokens for query while leveraging a light-weight QSM to encapsulate task-specific knowledge. This suggests that the significance of increasing model capacity in an appropriate way rather than simply increasing input tokens, is crutial in boosting model performance.

\input{exp_result/appendix_21k.tex}
\input{exp_result/appendix_head2toe.tex}

% VQT 246.95 samples/second
% SynQT 244.91
% VPT_deep 245.76
% VPT_Shallow 172.69
% bitfit 249.94

\section{Comparison between SynQT and Head2Toe}
We further provide the comparison with SynQT and Head2Toe on VTAB-1k with ViT-B/16 pre-trained on ImageNet-1K in Table  \ref{tab:head2toe}.
We further present a comparison between SynQT and Head2Toe on the VTAB-1k benchmark, using ViT-B/16 pre-trained on ImageNet-1K, as outlined in Table \ref{tab:head2toe}. Head2Toe is another method that utilizes intermediate representations for classification and simply applys an averaging over these features to reduce dimensionality. The input for Head2Toe consists of features from four distinct stages: after layer normalization, after the Multi-head Attention block, inside and after the MLP block, while VQT only utilizes the query output of the transformer blocks.

We observe a significant improvement in performance of SynQT from comparison with Head2Toe and VQT.
Specificly, SynQT outperforms both Head2Toe and VQT on 16 out of 19 tasks, indicating that
the intermediate representations of a task-specific synthesized query are more powerful than features derived from the original pre-trained model and random query output.
